# Supplementary material for: Beyond quasi-particle self-consistent $GW$ for molecules with vertex corrections
Source: arXiv:2412.01581 ancillary file (2025-02-11)
Supplement: Supplementary file 1 [file SI.pdf]

Supporting information to "Beyond quasi-particle self-consistent *GW* for molecules with vertex corrections"

Arno Förster<sup>1</sup>

*Theoretical Chemistry, Vrije Universiteit Amsterdam, De Boelelaan 1105,  
1081 HV Amsterdam, The Netherlands*

(\*Electronic mail: a.t.l.foerster@vu.nl)

(Dated: 2 December 2024)

## S1. CHARGED EXCITATION ENERGIES

TABLE S1. IPs, EAa, and fundamental gaps calculated with  $qs\Sigma^{BSE}@L^{BSE}$  using aug-cc-pvDZ and aug-cc-pVTZ basis sets. All values are in eV,

| Compound                 | aug-cc-pvDZ |       |       | aug-cc-pvTZ |       |       |
|--------------------------|-------------|-------|-------|-------------|-------|-------|
|                          | IP          | EA    | Gap   | IP          | EA    | Gap   |
| Acridine                 | 7.82        | 0.47  | 7.35  | –           | –     | –     |
| Anthracene               | 7.30        | 0.15  | 7.15  | –           | –     | –     |
| Azulene                  | 7.40        | 0.24  | 7.16  | 7.60        | 0.46  | 7.14  |
| Benzonitrile             | 9.78        | –0.44 | 10.22 | 9.97        | –0.28 | 10.25 |
| Benzoquinone             | 10.39       | 1.34  | 9.05  | 10.54       | 1.50  | 9.03  |
| Bodipy                   | 8.01        | 1.40  | 6.61  | –           | –     | –     |
| Cl4-benzoquinone         | 10.05       | 2.27  | 7.79  | 10.21       | 2.43  | 7.79  |
| Cl4-isobenzofuranedione  | 9.94        | 1.37  | 8.56  | –           | –     | –     |
| Dichlone                 | 9.76        | 1.68  | 8.08  | 9.90        | 1.87  | 8.03  |
| Dinitrobenzonitrile      | 11.06       | 1.54  | 9.52  | 11.24       | 1.74  | 9.50  |
| F4-benzenedicarbonitrile | 10.69       | 1.36  | 9.33  | 10.91       | 1.62  | 9.29  |
| F4-benzoquinone          | 11.00       | 2.10  | 8.90  | 11.16       | 2.29  | 8.87  |
| Fumaronitrile            | 11.12       | 0.78  | 10.34 | 11.34       | 1.00  | 10.34 |
| Maleicanhydride          | 11.42       | 0.76  | 10.65 | 11.61       | 0.98  | 10.63 |
| MDCNB                    | 10.26       | 0.37  | 9.90  | 10.46       | 0.57  | 9.90  |
| Naphthalenedione         | 9.85        | 1.26  | 8.59  | 9.98        | 1.40  | 8.58  |
| NDCA                     | 9.00        | 1.05  | 7.95  | –           | –     | –     |
| Nitrobenzene             | 10.13       | 0.29  | 9.85  | 10.31       | 0.48  | 9.83  |
| Nitrobenzonitrile        | 10.52       | 1.12  | 9.39  | 10.69       | 1.31  | 9.39  |
| Phenazine                | 8.25        | 0.88  | 7.37  | 8.37        | 1.02  | 7.35  |
| Phthalicanhydride        | 10.50       | 0.60  | 9.90  | 10.65       | 0.78  | 9.87  |
| Phthalimide              | 10.04       | 0.36  | 9.68  | 10.22       | 0.54  | 9.68  |
| TCNE                     | 11.66       | 2.89  | 8.78  | 11.89       | 3.14  | 8.75  |
| TCNQ                     | 9.29        | 3.30  | 5.99  | –           | –     | –     |

TABLE S2. IPs, EAa, and fundamental gaps calculated with qsGW@RPA using aug-cc-pvDZ and aug-cc-pVTZ basis sets. All values are in eV.

| Compound                | aug-cc-pvDZ |       |       | aug-cc-pvTZ |       |       |
|-------------------------|-------------|-------|-------|-------------|-------|-------|
|                         | IP          | EA    | Gap   | IP          | EA    | Gap   |
| Acridine                | 7.81        | 0.59  | 7.22  | 8.06        | 0.85  | 7.21  |
| Anthracene              | 7.30        | 0.25  | 7.05  | 7.52        | 0.49  | 7.03  |
| Azulene                 | 7.31        | 0.45  | 6.86  | 7.55        | 0.69  | 6.86  |
| Benzonitrile            | 9.73        | -0.38 | 10.11 | 9.96        | -0.13 | 10.09 |
| Benzoquinone            | 10.37       | 1.37  | 9.00  | 10.68       | 1.64  | 9.04  |
| Bodipy                  | 7.96        | 1.49  | 6.47  | 8.22        | 1.77  | 6.45  |
| Cl4-Benzoquinone        | 10.07       | 2.34  | 7.73  | 10.28       | 2.55  | 7.73  |
| Cl4-Isobenzofuranedione | 9.88        | 1.49  | 8.39  | 10.14       | 1.76  | 8.36  |
| Dichlone                | 9.73        | 1.76  | 7.97  | 9.95        | 1.98  | 7.97  |
| Dinitrobenzonitrile     | 10.98       | 1.64  | 9.34  | 11.20       | 1.88  | 9.32  |
| F4-Benzedicarbonitrile  | 10.59       | 1.48  | 9.11  | 10.83       | 1.77  | 9.06  |
| F4-Benzoquinone         | 11.02       | 2.15  | 8.86  | 11.28       | 2.42  | 8.85  |
| Fumaronitrile           | 11.23       | 0.76  | 10.47 | 11.46       | 1.03  | 10.43 |
| MaleicAnhydride         | 11.38       | 0.78  | 10.61 | 11.70       | 1.06  | 10.65 |
| mDCNB                   | 10.22       | 0.44  | 9.78  | 10.47       | 0.71  | 9.76  |
| Naphthalenedione        | 9.72        | 1.33  | 8.40  | 9.95        | 1.56  | 8.39  |
| NDCA                    | 8.94        | 1.13  | 7.81  | 9.20        | 1.40  | 7.80  |
| Nitrobenzene            | 10.01       | 0.38  | 9.63  | 10.24       | 0.66  | 9.58  |
| Nitrobenzonitrile       | 10.45       | 1.20  | 9.25  | 10.70       | 1.47  | 9.23  |
| Phenazine               | 8.24        | 1.02  | 7.23  | 8.50        | 1.28  | 7.22  |
| PhthalicAnhydride       | 10.36       | 0.69  | 9.67  | 10.59       | 0.95  | 9.64  |
| Phthalimide             | 9.90        | 0.44  | 9.45  | 10.13       | 0.70  | 9.43  |
| TCNE                    | 11.69       | 2.88  | 8.81  | 12.00       | 3.20  | 8.80  |
| TCNQ                    | 9.34        | 3.28  | 6.06  | 9.59        | 3.59  | 6.00  |

TABLE S3. IPs, EAa, and fundamental gaps calculated with  $qs\Sigma^{BSE}@L^{TDH}$  using aug-cc-pvDZ and aug-cc-pVTZ basis sets. All values are in eV.

| Compound                 | aug-cc-pvDZ |      |      | aug-cc-pvTZ |      |      |
|--------------------------|-------------|------|------|-------------|------|------|
|                          | IP          | EA   | Gap  | IP          | EA   | Gap  |
| Acridine                 | 7.62        | 1.09 | 6.54 | –           | –    | –    |
| Anthracene               | 7.15        | 0.76 | 6.39 | –           | –    | –    |
| Azulene                  | 7.17        | 0.92 | 6.26 | 7.39        | 1.14 | 6.24 |
| Benzonitrile             | 9.44        | 0.15 | 9.30 | 9.67        | 0.40 | 9.28 |
| Benzoquinone             | 9.68        | 1.96 | 7.71 | 9.97        | 2.21 | 7.76 |
| Bodipy                   | 7.66        | 1.80 | 7.71 | –           | –    | –    |
| Cl4-benzoquinone         | 9.60        | 2.88 | 6.73 | –           | –    | –    |
| Cl4-isobenzofuranedione  | 9.51        | 1.94 | 7.56 | –           | –    | –    |
| Dichlone                 | 9.33        | 2.25 | 7.07 | –           | –    | –    |
| Dinitrobenzonitrile      | 10.56       | 2.17 | 8.39 | –           | –    | –    |
| F4-benzenedicarbonitrile | 10.15       | 1.94 | 8.21 | 10.46       | 2.30 | 8.16 |
| F4-benzoquinone          | 10.49       | 2.61 | 7.88 | 10.82       | 2.97 | 7.85 |
| Fumaronitrile            | 10.87       | 1.37 | 9.51 | 11.16       | 1.62 | 9.54 |
| Maleicanhydride          | 10.78       | 1.25 | 9.53 | 11.11       | 1.50 | 9.61 |
| MDCNB                    | 9.94        | 0.98 | 8.96 | 10.20       | 1.26 | 8.93 |
| Naphthalenedione         | 9.40        | 1.83 | 7.56 | –           | –    | –    |
| NDCA                     | 8.69        | 1.62 | 7.07 | –           | –    | –    |
| Nitrobenzene             | 9.71        | 0.96 | 8.75 | 9.94        | 1.25 | 8.69 |
| Nitrobenzonitrile        | 10.01       | 1.70 | 8.32 | 10.27       | 2.01 | 8.26 |
| Phenazine                | 8.03        | 1.55 | 6.49 | –           | –    | –    |
| Phthalicanhydride        | 9.93        | 1.24 | 8.70 | 10.16       | 1.50 | 8.66 |
| Phthalimide              | 9.59        | 0.97 | 8.63 | 9.82        | 1.25 | 8.57 |
| TCNE                     | 11.34       | 3.27 | 8.06 | –           | –    | –    |
| TCNQ                     | 8.99        | 3.59 | 5.40 | –           | –    | –    |

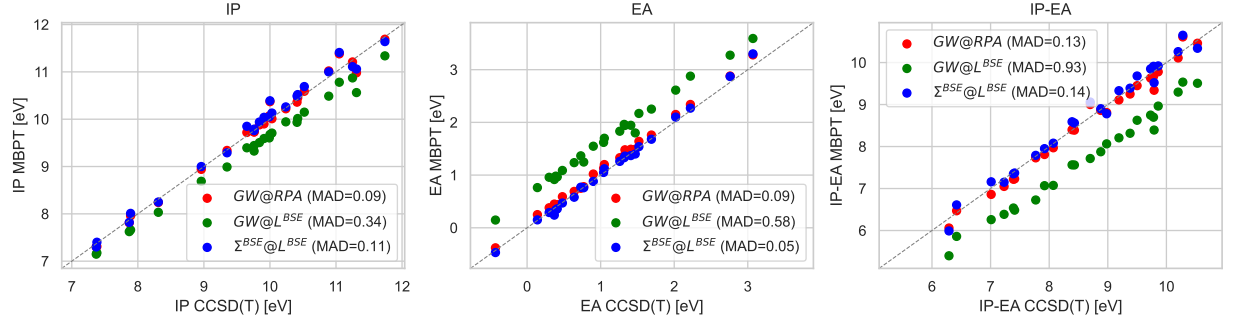

FIG. S1. Deviations of the molecules in the ACC24 set to  $\Delta\text{CCSD(T)}$  for quasi-particle self-consistent  $\text{GW@RPA}$ ,  $\text{GW@L}^{BSE}$  and  $\Sigma^{BSE}@L^{BSE}$  for IPs (left), EAs (middle) and fundamental gaps (right). All values are in eV. All values, including the reference values,<sup>1</sup> have been calculated using the aug-cc-pvDZ basis set.

## S2. NEUTRAL EXCITATION ENERGIES

TABLE S4: BSE@qsGW and  $qs\Sigma^{BSE}@L^{BSE}$  neutral excitations for the QUEST#6 database.<sup>2</sup> The TBE (theoretical best estimate) values correspond to the ones calculated at cc-pVTZ.<sup>2</sup> All values are in eV.

| Molecule                  | Transition                        | BSE@qsGW |      |      | qsΣ <sup>BSE</sup> @L <sup>BSE</sup> |      |      |      | Primary contribution      |
|---------------------------|-----------------------------------|----------|------|------|--------------------------------------|------|------|------|---------------------------|
|                           |                                   | TBE      | TZP  | TZ2P | TZ3P                                 | TZP  | TZ2P | TZ3P |                           |
| Aminobenzonitrile         | <sup>1</sup> A <sub>1</sub> (CT)  | 5.26     | 5.08 | 5.08 | 5.07                                 | 5.31 | 5.31 | –    | 4B2 → 5B2                 |
| Aniline                   | <sup>1</sup> A <sub>1</sub> (CT)  | 5.87     | 5.62 | 5.60 | 5.56                                 | 5.92 | 5.91 | –    | 3b2 → 2a2, 1a2 → 4b2      |
| Azulene                   | <sup>1</sup> A <sub>1</sub> (CT)  | 3.89     | 3.47 | 3.44 | 3.44                                 | 3.87 | 3.85 | 3.83 | 2a2 → 3a2, 3b2 → 4b2      |
|                           | <sup>1</sup> B <sub>2</sub> (CT)  | 4.55     | 4.43 | 4.41 | 4.41                                 | 4.93 | 4.93 | 4.90 | 3b2 → 3a2                 |
| Benzonitrile              | <sup>1</sup> A <sub>2</sub> (CT)  | 7.10     | 6.91 | 6.83 | 6.83                                 | 6.91 | 6.84 | 6.81 | 8B1 → 4B2                 |
| Benzothiadiazole          | <sup>1</sup> B <sub>2</sub> (CT)  | 4.37     | 4.01 | 3.98 | 3.93                                 | 4.26 | 4.21 | –    | 2a2 → 5b1                 |
| β-Dipeptide               | <sup>1</sup> A′(CT)               | 8.51     | 8.66 | –    | –                                    | 8.58 | –    | –    | 7a// → 10a//, 7a// → 9a// |
|                           | <sup>1</sup> A″(CT)               | 8.90     | 8.89 | –    | –                                    | 8.65 | –    | –    | 31a′ → 9a//, 30a′ → 10a// |
| Dimethylaminobenzonitrile | <sup>1</sup> A <sub>1</sub> (CT)  | 4.94     | 4.85 | 4.85 | –                                    | 5.03 | 5.03 | –    | 5b2 → 6b2                 |
| Dimethylaniline           | <sup>1</sup> B <sub>2</sub> (CT)  | 4.47     | 4.54 | 4.54 | –                                    | 4.81 | 4.81 | –    | 4B2 → 3A2                 |
|                           | <sup>1</sup> A <sub>1</sub> (CT)  | 5.54     | 5.39 | 5.38 | –                                    | 5.65 | 5.65 | –    | 4B2 → 5B2                 |
| Dipeptide                 | <sup>1</sup> A″(CT)               | 8.15     | 8.53 | –    | –                                    | 8.43 | –    | –    | 28a′ → 8a//, 28a′ → 9a//  |
| N-Phenylpyrrole           | <sup>1</sup> B <sub>2</sub> (CT)  | 5.53     | 5.33 | 5.31 | –                                    | 5.50 | 5.49 | –    | 2a2 → 3a2                 |
|                           | <sup>1</sup> A <sub>1</sub> (CT)  | 6.04     | 6.09 | 6.08 | –                                    | 6.31 | 6.28 | –    | 2a2 → 5b2                 |
| Nitroaniline              | <sup>1</sup> A <sub>1</sub> (CT)  | 4.57     | 4.37 | 4.34 | 4.31                                 | 4.64 | 4.63 | –    | 4B2 → 5B2                 |
| Nitrodimethylaniline      | <sup>1</sup> A <sub>1</sub> (CT)  | 4.28     | 4.13 | 4.10 | –                                    | 4.35 | 4.34 | –    | 5B2 → 6B2                 |
| Phthalazine               | <sup>1</sup> A <sub>2</sub> (CT)  | 3.93     | 4.10 | 4.07 | 4.02                                 | 4.37 | 4.31 | 4.32 | 13B2 → 4B1                |
|                           | <sup>1</sup> B <sub>1</sub> (CT)  | 4.34     | 4.46 | 4.42 | 4.37                                 | 4.87 | 4.81 | 4.79 | 13B2 → 3A2                |
| Quinoxaline               | <sup>1</sup> B <sub>2</sub> (CT)  | 4.74     | 4.37 | 4.36 | 4.32                                 | 4.65 | 4.65 | 4.62 | –                         |
|                           | <sup>1</sup> A <sub>1</sub> (CT)  | 5.75     | 5.72 | 5.70 | 5.68                                 | 6.12 | 6.10 | 6.09 | –                         |
|                           | <sup>1</sup> B <sub>1</sub> (CT)  | 6.33     | 6.10 | 6.07 | 6.05                                 | 6.49 | 6.47 | 6.44 | –                         |
| Twisted DMABN             | <sup>1</sup> A <sub>2</sub> (CT)  | 4.17     | 4.18 | 4.19 | –                                    | 4.37 | 4.35 | –    | 10B1 → 8B2                |
|                           | <sup>1</sup> B <sub>1</sub> (CT)  | 4.84     | 4.97 | 4.97 | –                                    | 5.16 | 5.15 | –    | 10B1 → 3A2                |
| Twisted PP                | <sup>1</sup> 2B <sub>2</sub> (CT) | 5.73     | 5.83 | 5.82 | –                                    | 6.00 | 5.89 | –    | 2A2 → 3A2                 |
|                           | <sup>1</sup> 2A <sub>1</sub> (CT) | 5.82     | 6.04 | 6.03 | –                                    | 6.25 | 6.01 | –    | 9B1 → 9B2                 |
| Nitropyridine N-Oxide     | <sup>1</sup> 2A <sub>1</sub> (CT) | 4.24     | 3.94 | 3.93 | 3.92                                 | 4.36 | 4.39 | 4.30 | 4B2 → 5B2                 |
| Nitrobenzene              | <sup>2</sup> A <sub>1</sub>       | 5.57     | 5.23 | 5.18 | 5.16                                 | 5.54 | 5.53 | –    | 3b2 → 4b2                 |

TABLE S5. Comparison of the lowest 5 excitation energies of Benzonitrile and Quinoxaline calculated with the cc-pVTZ and the TZ3P basis sets.

| <b>Excitation</b>   | <b>TZ2P</b> | <b>cc-pVTZ</b> | <b>Diff</b> |
|---------------------|-------------|----------------|-------------|
| <b>Benzonitrile</b> |             |                |             |
| 1                   | 5.38        | 5.37           | 0.01        |
| 2                   | 5.89        | 5.89           | -0.01       |
| 3                   | 6.81        | 6.79           | 0.02        |
| 4                   | 6.96        | 6.97           | -0.01       |
| 5                   | 6.98        | 7.01           | -0.03       |
| <b>Quinoxaline</b>  |             |                |             |
| 1                   | 4.07        | 4.05           | -0.02       |
| 2                   | 4.62        | 4.60           | -0.02       |
| 3                   | 4.69        | 4.66           | -0.02       |
| 4                   | 5.50        | 5.46           | -0.03       |
| 5                   | 5.98        | 5.98           | 0.00        |

## REFERENCES

- <sup>1</sup>R. M. Richard, M. S. Marshall, O. Dolgounitcheva, J. V. Ortiz, J. L. Brédas, N. Marom, and C. D. Sherrill, “Accurate Ionization Potentials and Electron Affinities of Acceptor Molecules I. Reference Data at the CCSD(T) Complete Basis Set Limit,” *J. Chem. Theory Comput.* **12**, 595–604 (2016).
- <sup>2</sup>P. F. Loos, M. Comin, X. Blase, and D. Jacquemin, “Reference Energies for Intramolecular Charge-Transfer Excitations,” *J. Chem. Theory Comput.* **17**, 3666–3686 (2021), arXiv:2103.02947.
